# Supplementary material for: Magnetization density distribution of Sr$_2$IrO$_4$: Deviation from a local $j_\text{eff}=1/2$ picture
Source: arXiv:1904.09139 source file (2020-08-14)
Supplement: Supplementary file 1 [file Sr2IrO4-MD-v8-supp.pdf]

# **Supplementary information**

## **Magnetization density distribution in $\text{Sr}_2\text{IrO}_4$ : Deviation from a local $j_{\text{eff}} = 1/2$ picture**

### **Contents**

|          |                                                                     |           |
|----------|---------------------------------------------------------------------|-----------|
| <b>1</b> | <b>Sample preparation and characterization</b>                      | <b>2</b>  |
| <b>2</b> | <b>Polarized neutron diffraction</b>                                | <b>4</b>  |
| <b>3</b> | <b>Data treatment with two magnetic field orientations</b>          | <b>6</b>  |
| <b>4</b> | <b>Analysis using the maximum entropy method</b>                    | <b>7</b>  |
| <b>5</b> | <b>Analysis using a multipole expansion model</b>                   | <b>10</b> |
| <b>6</b> | <b>Theoretical modeling of <math>\text{Sr}_2\text{IrO}_4</math></b> | <b>17</b> |
| <b>7</b> | <b>References</b>                                                   | <b>22</b> |

# 1 Sample preparation and characterization

High-quality single crystals of  $\text{Sr}_2\text{IrO}_4$  were grown at Laboratoire de Physique des Solides at Orsay using a self-flux method in the platinum crucibles. The temperature dependence of the uniform magnetization was measured using a SQUID under a magnetic field of  $H = 1$  T along the  $[110]$  (Fig. **S1a**).  $\text{Sr}_2\text{IrO}_4$  undergoes a canted antiferromagnetic (AFM) transition. The ordered AFM moment is found to be about  $0.21 \mu_B/\text{Ir}^2$  or about  $0.36 \mu_B/\text{Ir}^3$  by single crystal neutron diffraction. We here discussed the weak in-plane ferromagnetic moment due to the moment canting (see Fig 1.b). In presence of the magnetic field above  $H > 0.2$  T, the system exhibits a ferromagnetic component at  $T \approx 235$  K, where the derivative  $dM/dT$  diverges. The saturation weak ferromagnetic (WFM) moment is  $\approx 0.08 \mu_B/\text{Ir}$  at  $T = 10$  K. It is well consistent with the reported value for single crystals grown under the best conditions <sup>1</sup>. For the polarized neutron diffraction measurements, which require a large amount of the sample, 50 single crystals of a small size (typically  $< 2 \times 1 \times 0.2 \text{ mm}^3$ ) were coaligned within a diameter of 10 mm on an aluminum plate (Fig. **S1b**).

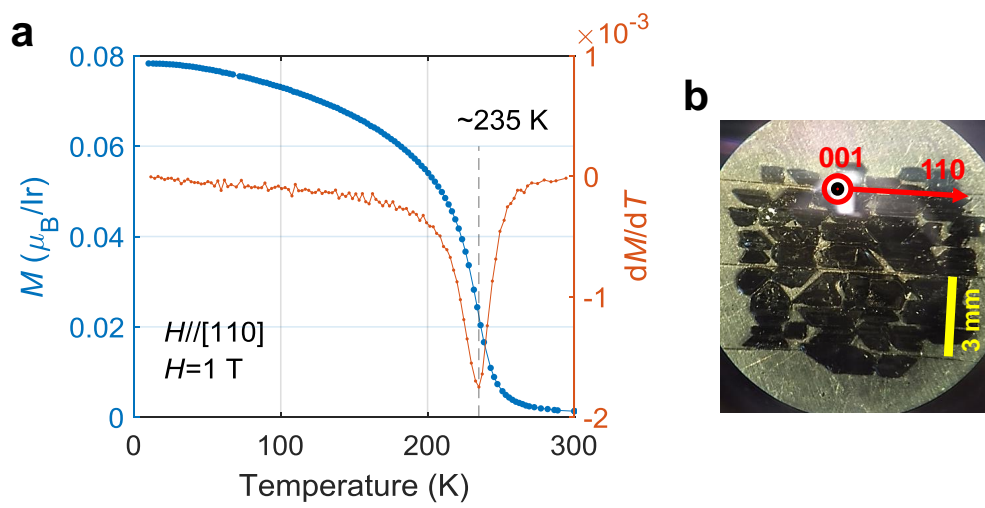

Figure **S1**: (a) Temperature dependence of the uniform magnetization and its derivative measured by a SQUID. (b) Coaligned 50 single crystals on an aluminum plate.

## 2 Polarized neutron diffraction

Polarized neutron diffraction (PND) measurements were performed on three different polarized neutron diffractometers, *5C1* and *6T2* at the *ORPHÉE* reactor (LLB CEA Saclay), and *POLI* at *FRM-II* ((Maier-Leibnitz Zentrum Garching). Thermal and hot polarized neutron wavelengths were used with  $\lambda=1.4$  Å (*6T2*), 1.15 Å (*POLI*) and 0.84 Å (*5C1*). A vertical uniform magnetic field of 5 T on *5C1/6T2@LLB* and 2.2 T on *POLI@FRMII* has been applied at the sample position. As the weak ferromagnetic component saturates above  $\sim 1$  T, that difference between the applied fields is not significant. The temperature was set at 4 K in the antiferromagnetic state of  $\text{Sr}_2\text{IrO}_4$ .

Incoming neutrons were polarized by a Heusler alloy monochromator, a supermirror bender or a  $^3\text{He}$  filter. The direction of incident neutron polarization – spin-up or spin-down – was chosen by a polarization flipper. The incident spin-polarized neutrons are scattered by the nuclei and by the local magnetization, which are denoted by nuclear and magnetic scattering, respectively. The total neutron cross section for a non-chiral system is given by

$$\sigma = F_N F_N^* + \mathbf{M}_\perp \cdot \mathbf{M}_\perp^* + \mathbf{P}_i \cdot (\mathbf{M}_\perp F_N^* + \mathbf{M}_\perp^* F_N), \quad (\text{S1})$$

where  $F_N$  is the nuclear structure factor,  $\mathbf{M}_\perp$  is the magnetic interaction vector and  $\mathbf{P}_i$  is the incident neutron polarization vector. The magnetic interaction vector is given as  $\mathbf{M}_\perp = \hat{Q} \times F_M(\mathbf{Q}) \times \hat{Q}$  with the scattering vector  $\mathbf{Q}$  and  $F_M(\mathbf{Q})$  the magnetic structure factor, *i.e.*, the Fourier transform of the magnetic moment distribution. Therefore, only magnetic components perpendicular to the scattering vector participate in the magnetic scattering. The last *magnetic-nuclear interference*

term appears only for a polarized beam ( $|P_i| > 0$ ), and it contributes to the scattering for a mixed nuclear-magnetic Bragg reflection with propagation vector  $\mathbf{q} = 0$ . It corresponds to the magnetic response at the Brillouin zone center,  $\Gamma$  point that would differ from the magnetic response at the antiferromagnetic propagation wave vector. In all the manuscript, we are only speaking about the weak ferromagnetic component of the moment.

In case of PND where incoming neutron polarization is directed parallel or antiparallel to an external magnetic field, one measures the intensity of the scattered neutrons for the two states of the flipper. We note that no final polarization analysis is performed. Therefore, the measured intensity, obtained for each state of the flipper, is written as a function of the real structure factors,

$$\begin{aligned} I_{\uparrow} &= F_N^2 + M_{\perp}^2 + 2P_i F_N M_{\perp} \\ I_{\downarrow} &= F_N^2 + M_{\perp}^2 - 2P'_i F_N M_{\perp}, \end{aligned} \tag{S2}$$

where  $M_{\perp}$  is now the projection of the magnetic interaction vector  $\mathbf{M}_{\perp}$  along the polarization vector  $\mathbf{P}_i$  with  $P_i$  and  $P'_i$  being the incident polarization for spin-up and spin-down, respectively. The PND measurement is thus only sensitive to the uniform magnetization along the applied magnetic field. Note that  $I_{\uparrow} \sim |F_N + M_{\perp}|^2$  and  $I_{\downarrow} \sim |F_N - M_{\perp}|^2$  when  $P_i \approx 1$ . Using  $P_i = p$ ,  $P'_i = pe$  and  $M_{\perp} = \sin \alpha F_M$  where  $\alpha$  is the angle between the magnetic interaction vector and the scattering vector, the flipping ratio is given as Eq. (2) in the main text with the polarization efficiency  $p$  of the polarizer and the flipping efficiency  $e$  of the flipper.

### 3 Data treatment with two magnetic field orientations

The flipping ratios were measured at a number of Bragg reflections with two different sample orientations with respect to the applied magnetic field:  $H \parallel [010]$  and  $H \parallel [\bar{1}10]$ . The magnetic structure factors at common reflections such as  $(0, 0, l)$ ,  $(2, 0, l)$  and  $(2, 2, l)$  are shown for each orientation in Fig. S2. It is important to notice that the scaling for both orientations is the same and it is consistent to macroscopic SQUID measurements, which show the same saturation magnetic moment for a magnetic field along the two directions. It also supports an isotropic WFM moment, which follows the applied magnetic field <sup>4,5</sup>. We therefore have combined and taken an average of two data sets without an additional scaling.

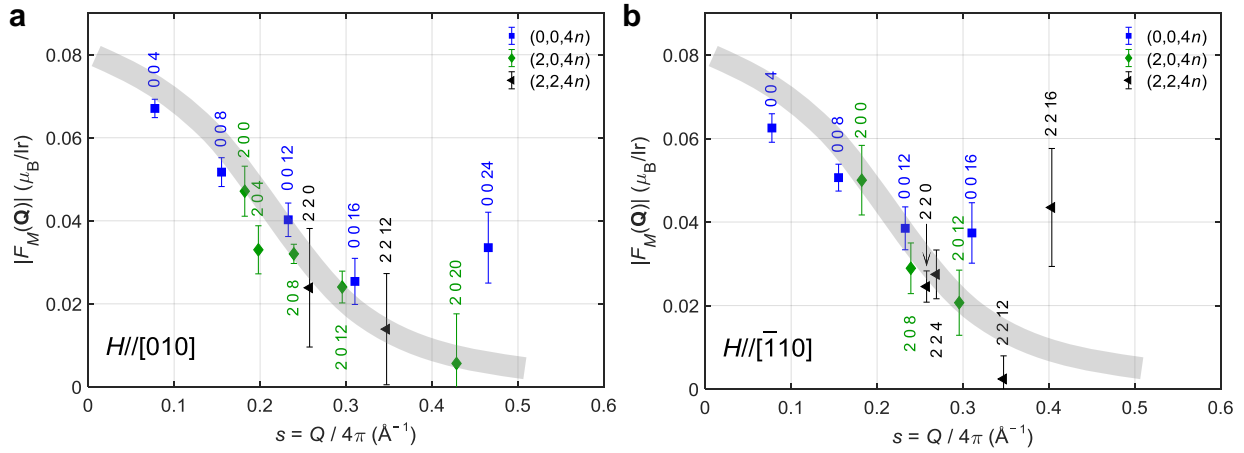

Figure S2: Measured magnetic structure factors with a magnetic field along (a)  $H \parallel [010]$  and (b)  $H \parallel [\bar{1}10]$ .

## 4 Analysis using the maximum entropy method

We have tested the maximum entropy method (MEM) by changing the initial positive and negative magnetic moments. The resulting positive and negative magnetic moments are limited by the initial values, thus they are starting points for fitting and also serve as upper bounds. The difference between positive and negative moments was set to the net unit cell magnetic moment,  $0.64\mu_B$  (8 times  $0.08\mu_B/\text{Ir}$ ). As seen in Fig. S3a, the agreement factor defined by  $R_w = \sum (|F_{\text{obs}} - F_{\text{calc}}| / \sigma_F) / \sum (|F_{\text{obs}}| / \sigma_F)$  is poor ( $\approx 15\%$ ) for only a small negative moment being allowed. It decreases rapidly as the initial negative moment increases, and it is saturated with twice better  $R_w \approx 8\%$  for a significant negative moment above  $0.25\mu_B$ . Initial values larger than  $0.3\mu_B$ , however, do not improve the agreement factor any more and the resulting negative moment either does not follow the initial value. Instead, the both positive and negative densities spread out so the density distribution is only dispersed while the spatial features are unchanged as shown in Fig. S4c,f. Therefore, we have chosen  $+0.94\mu_B$  and  $-0.30\mu_B$  as optimized initial positive and negative moments, and the resulting moments are  $+0.93\mu_B$  ( $+0.116\mu_B/\text{Ir}$ ) and  $-0.29\mu_B$  ( $-0.036\mu_B/\text{Ir}$ ), respectively. The calculated magnetic structure factors from the optimized MEM result ( $R_w \approx 8\%$ ) are shown with measured ones in Fig. S3b

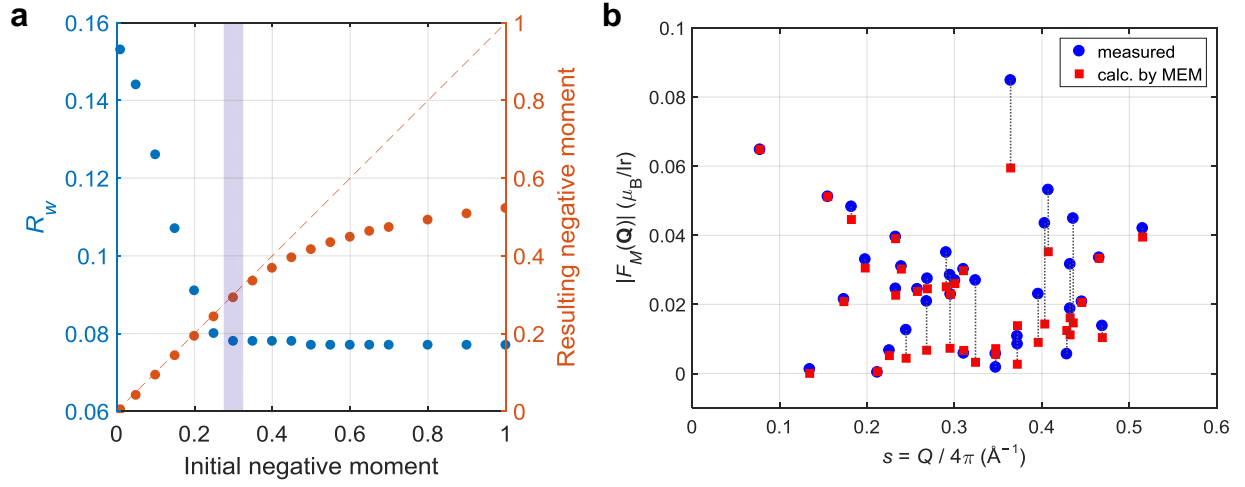

Figure **S3**: (a) Agreement factor  $R_w$  and resulting negative moment per unit cell versus the initial value for negative moment for the MEM analysis. (b) Measured and calculated magnetic structure factors  $|F_M(\mathbf{Q})|$  for the optimized MEM result.

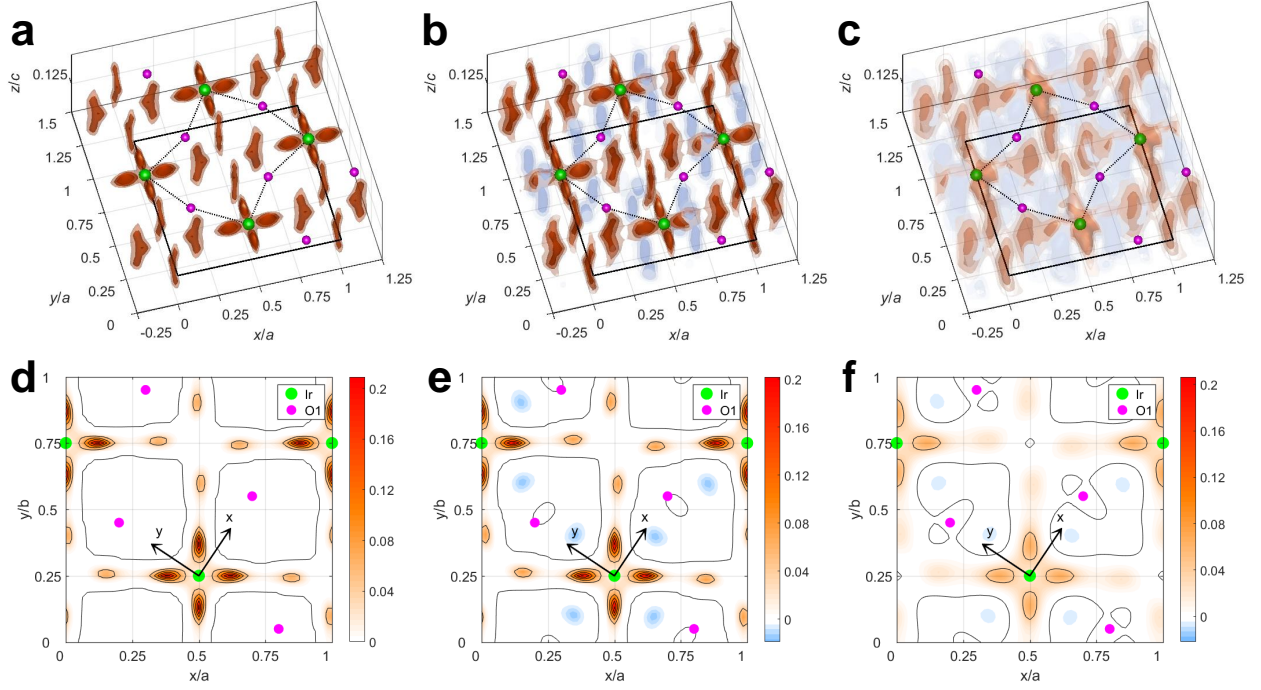

**Figure S4:** 3D magnetization density distribution on the  $z = c/8$  layer reconstructed by the MEM analysis with the initial negative moment (a)  $-0.01$ , (b)  $-0.30$ , and (c)  $-0.70 \mu_B$  per unit cell. Isosurfaces encompassing 30%, 50% and 70% of the volume density are plotted with a descending opacity according to their isovalues. Red and blue surfaces denote positive and negative magnetizations, respectively. The solid square and dotted lines denote the unit cell and Ir-O bonds, respectively. (d-f) Sliced density contour maps at  $(x, y, c/8)$  for the given initial negative moment in (a-c). The contour step is  $0.04 \mu_B / \text{\AA}^3$ . The black arrows correspond to the Ir-O bonding directions tilted by  $11^\circ$  from the crystallographic tetragonal axes.

## 5 Analysis using a multipole expansion model

The magnetization density can be modeled by a superposition of spherical harmonic density functions, known as the *multipolar expansion*<sup>6,7</sup>:

$$m(\mathbf{r}) = \sum_{\text{atoms}} \sum_{l=0}^{\infty} R_n^2(r) \sum_{m=-l}^l p_{l,m} y_{l,m}(\theta, \phi), \quad (\text{S3})$$

where  $R_n(r)$  are radial wave functions,  $y_{l,m}(\theta, \phi)$  are angular density functions, and  $p_{l,m}$  are population coefficients. Simple normalized, Slater-type nodeless radial wave functions  $R_n(r)$  are defined as:

$$R_n(r) = \sqrt{\frac{(2\zeta)^{2n+1}}{(2n)!}} r^{n-1} \exp(-\zeta r),$$

with  $n = 5$  chosen for the  $5d$ -orbitals. The angular density functions  $y_{l,m}(\theta, \phi)$  are the real-valued spherical harmonic functions:

$$y_{l,m}(\theta, \phi) = N_{l,m} P_l^{|m|}(\cos \theta) \begin{cases} \cos m\phi & \text{for } m > 0 \\ \sin |m|\phi & \text{for } m < 0, \end{cases}$$

where  $P_l^m$  are the associated Legendre polynomials and  $N_{l,m}$  are the normalization factors<sup>8</sup> satisfying

$$\int |y_{l,m}| d\Omega = \begin{cases} 1 & \text{for } l = 0 \\ 2 & \text{for } l > 0. \end{cases}$$

Note that these angular *density* functions are distinct from the angular *wave*-functions,  $Y_l^m$ , which are complex-valued and have a different normalization condition,  $\int |Y_l^m|^2 d\Omega = 1$ .

The magnetic form factors corresponding to the model magnetization density in Eq. (S3) become

$$f(\mathbf{Q}) = \sum_{l=0}^{\infty} \phi_l(Q) \sum_{m=-l}^l p_{l,m} y_{l,m}(\theta_k, \phi_k)$$

with

$$\phi_l(Q) = 4\pi i^l \int_0^{\infty} R_n^2(r) j_l(Qr) r^2 dr,$$

where  $j_l$  is a spherical Bessel function of order  $l$ . Then the least-squares refinement with the measured  $F_M$  was done using the MPLSQ program<sup>9</sup>. For the refinement, the total magnetic moment is constrained:  $\mu_{\text{Ir}} + 2\mu_{\text{O1}} + 2\mu_{\text{O2}} = 0.08\mu_{\text{B}}/\text{Ir}$ .

The multipole density functions allowed by the point group  $D_{4h}$  ( $4/mmm$ ) are shown in Fig. S5a. Because the spherical harmonic functions constitute a complete set in the spherical harmonic point group, the orbital density distribution given by a square of wave function  $|Y_l^m|^2$  must be a linear combination of spherical harmonic density functions  $y_{l,m}$ <sup>7</sup>. The orbital-multipole relations for the point group  $D_{4h}$  are defined as  $p_l^m |Y_l^m|^2 = p_{i,j} y_{i,j}$  with

$$\begin{pmatrix} p_2^0 \\ p_2^{\pm 1} \\ p_2^2 \\ p_2^{-2} \end{pmatrix} = \begin{pmatrix} 0.200 & 1.039 & 1.396 & 0.000 \\ 0.200 & 0.520 & -0.931 & 0.000 \\ 0.200 & -1.039 & 0.233 & 1.570 \\ 0.200 & -1.039 & 0.233 & -1.570 \end{pmatrix} \begin{pmatrix} p_{0,0} \\ p_{2,0} \\ p_{4,0} \\ p_{4,4} \end{pmatrix}.$$

The  $d$  orbital densities reconstructed using the spherical density functions are also shown in Fig. S5b. Using this orbital-multipole relations, the orbital populations were obtained from the fitted density function populations.

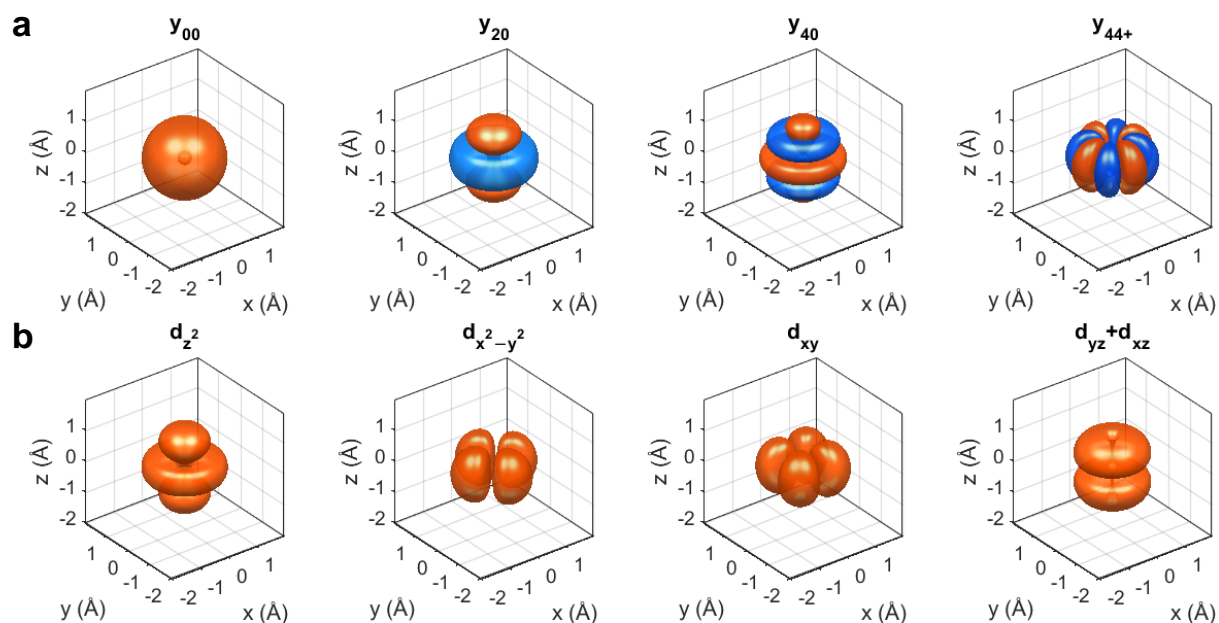

Figure S5: (a) Multipole density functions allowed by  $4/mmm$  symmetry. Red and blue surface denote positive and negative density, respectively. (b) Density distribution of  $d$  orbitals constructed by a linear combination of multipole density functions.

In order to describe the large spatial extent of the positive magnetization density, the radial wave function was also examined. It is clear as shown in Fig. S6d that the theoretical radial function with the radial exponent  $\zeta = 3.74$  is not fit well ( $R_w \approx 22\%$ ) with the measured magnetic structure factor and also not able to describe the wide spatial extent found by the MEM analysis. The best value  $\zeta = 2.7$  for a single radial exponent was also refined, but the agreement factor was not improved significantly ( $R_w \approx 18\%$ ) as shown in Fig. S7. Therefore, we introduced an additional radial exponent. The radial wave function with two radial exponents provides significantly better agreement ( $R_w \approx 9\%$ ) with measured magnetization density and describes the large extent of observed magnetization density as shown in Fig. S6f.

In order to examine a possible magnetization density expected from a strong  $d$ - $p$  hybridization at the oxygen site, the refinements with a spherical magnetization density at the O1 and O2 sites were also performed. However, the agreement factor did not become better and also the refined magnetization density at the O sites is statistically negligible.

We have also examined to fit the data with actual orbital density functions instead of multipole density functions. When all possible  $5d$  orbitals are allowed, it obviously gives the same result ( $R_w \approx 9\%$ ) with similar population of each orbitals as shown in Fig. S8a. In addition, as it is known to consist mostly of  $t_{2g}$  orbitals, the model fit allowing only  $d_{xy}$ ,  $d_{yz}$ ,  $d_{xz}$  orbitals was also performed. As shown in Fig. S8b, the negative magnetic density with  $d_{x^2-y^2}$  symmetry disappears as expected, but the agreement becomes twice worse ( $R_w \approx 17\%$ ). Therefore, we conclude that the observed magnetic octapolar shape, mainly from  $y_{44+}$  angular density function, is essential to

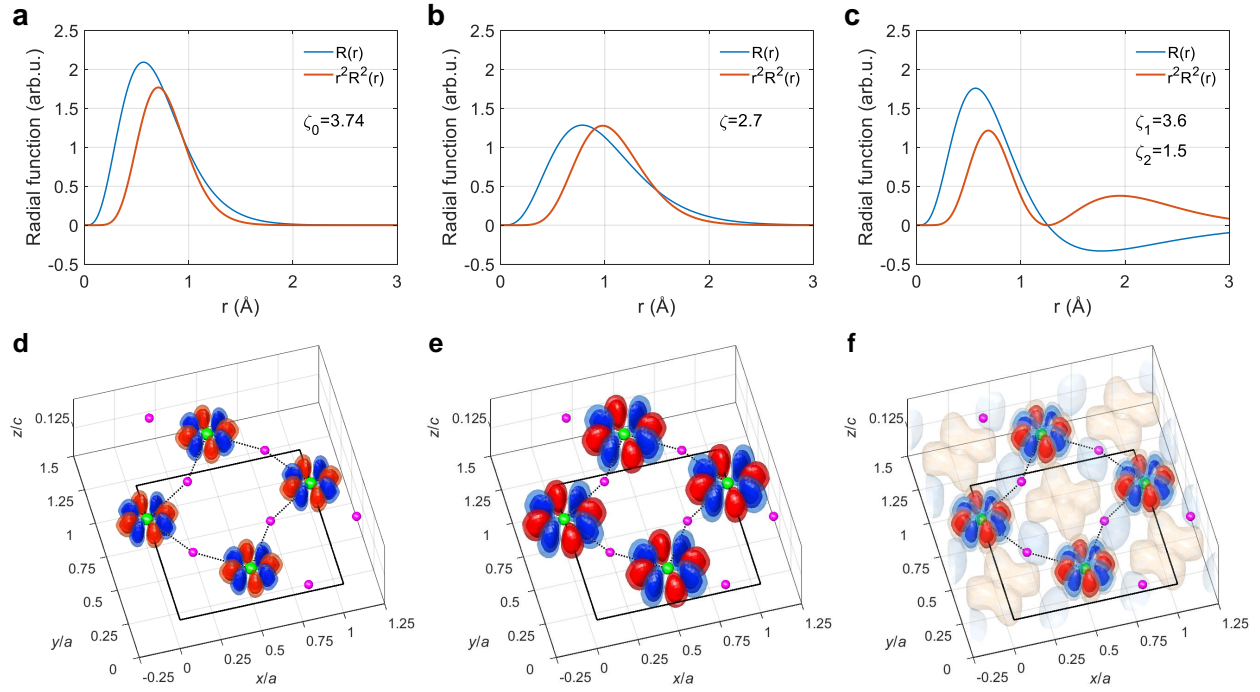

Figure S6: Radial wave functions  $R(r)$  and radial distribution functions  $r^2 R^2(r)$  with (a) the theoretical radial exponent for isolated Ir atoms, (b) an optimized single radial exponent, and (c) double radial exponents. (d-f) Reconstructed magnetization density distributions with different radial wave functions in (a-c).

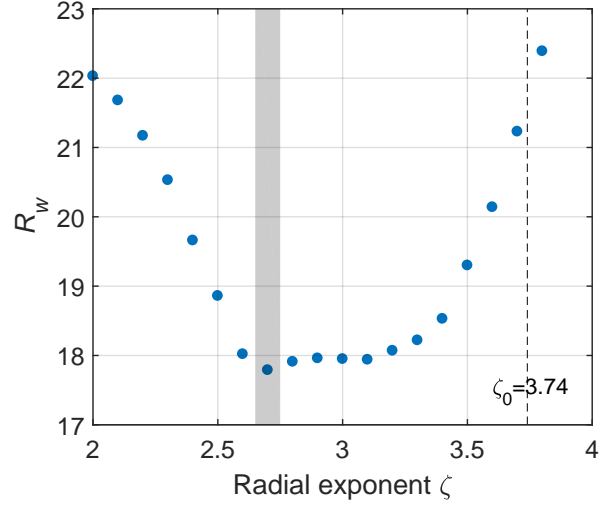

Figure **S7**: Agreement factor  $R_w$  versus the radial exponent  $\zeta$  for the multipole expansion model with a single radial exponent. The agreement factor decreases by  $\sim 20\%$  at  $\zeta \approx 2.7$  compared with the theoretical radial exponent  $\zeta_0 = 3.74$ .

describe our measured data.

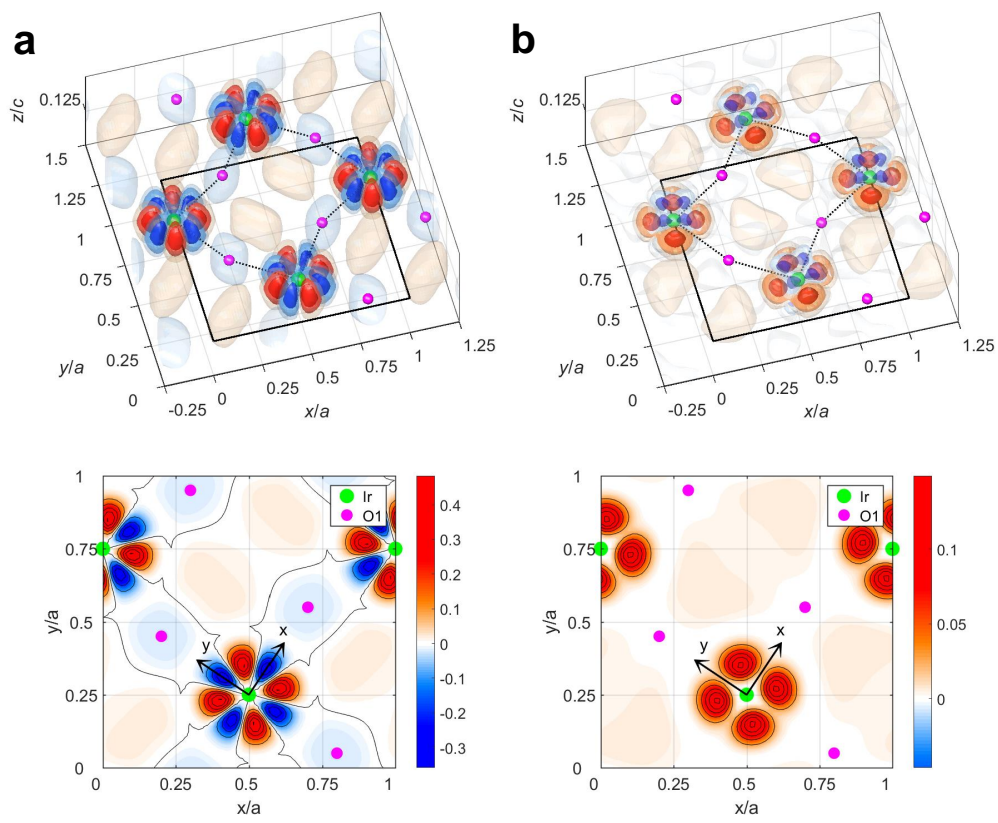

Figure S8: Magnetization density distribution obtained by orbital density model fit with (a) all five  $d$  orbitals and (b) only three  $t_{2g}$  orbitals.

## 6 Theoretical modeling of $\text{Sr}_2\text{IrO}_4$

In order to understand the puzzling magnetization density distribution of  $\text{Sr}_2\text{IrO}_4$  we propose a modelization based on a multi-orbital generalization of the Heisenberg-model. The Heisenberg model can be understood as a lowest-order expansion in the ratio between hopping and Coulomb interaction around a localized electronic state in a half-filled periodic lattice system. Here, this simple philosophy becomes more subtle due to the spin-orbital entangled nature of the localized hole state.

Let us denote by  $\varphi_{\mathbf{k},\alpha} = \sum_{(l,\sigma)} S(\mathbf{k})_{\alpha,(l\sigma)} \chi_{\mathbf{k}(l\sigma)}$  a Wannier representation of the  $t_{2g}$  manifold chosen such that the hole resides fully in the upmost (two-fold degenerate) state, which we will denote in the following as  $\varphi_{\mathbf{k},1/2,m_j}$ ,  $m_j = \pm 1/2$ . Here,  $\chi_{\mathbf{k}(l\sigma)}$  denotes the Fourier transform of a tensor product of a Wannier function of dominant cubic harmonic character  $l$  and a spin state  $\sigma$ . Importantly, the transformation  $S$  between the cubic harmonic basis and the effective  $\alpha = 1/2$  and  $\alpha = 3/2$  Wannier states is  $\mathbf{k}$ -dependent. This means that it does not only deviate from the standard isotropic  $\frac{1}{\sqrt{3}} : \frac{1}{\sqrt{3}} : \frac{1}{\sqrt{3}}$  composition of  $t_{2g}$  orbitals, but in particular does so in a momentum-dependent fashion, in accordance with ab initio calculations<sup>10</sup> and recent photoemission experiments<sup>11,12</sup>.

In real space, the hole has a representation by creation and annihilation operators

$$d_{i,1/2,m_j}^{(\dagger)} = \sum_{i',(l,\sigma)} S(R_i - R_{i'})_{(1/2\ m_j),(l\sigma)}^{(\dagger)} d_{i',(l\sigma)}^{(\dagger)}. \quad (\text{S4})$$

The Heisenberg-model construction then proceeds in this basis to second order in the hopping

yielding a Hamiltonian of the form

$$\mathcal{H} = \sum_{n, \tilde{n}} \sum_{i', i'', j', j''} \sum_{l, l', \tilde{l}, \tilde{l}'} \tilde{J}_{(i', i'', l, l'), (j', j'', \tilde{l}, \tilde{l}')}^{(n, \tilde{n})} S_{i', i''}^{l, l' (n)} S_{j', j''}^{\tilde{l}, \tilde{l}' (\tilde{n})}, \quad (\text{S5})$$

where  $i', i'', j', j''$  denote sites on the lattice,  $l, l', \tilde{l}, \tilde{l}'$  orbitals on these sites in a basis of cubic harmonics and  $n, \tilde{n}$  the index of Pauli spin matrices,  $\tau_{\sigma\sigma'}^{(n)}$ . Here, we defined the generalized spin operator

$$S_{i', i''}^{l, l' (n)} = \sum_{\sigma, \sigma'} d_{i'l\sigma}^\dagger \tau_{\sigma\sigma'}^{(n)} d_{i''l'\sigma'}. \quad (\text{S6})$$

This cumbersome object is a direct generalization to spin-orbit space of the multi-orbital  $t$ - $J$ -model that has been derived for the iron pnictides<sup>13</sup>, considered in the special case of half-filling.

In the following, we inspect the diagonal terms in site and orbital space of the tensor  $\tilde{\mathbf{J}}$

$$\mathcal{H} = \sum_{n, \tilde{n}} \sum_{i', j'} S_{i', l}^{(n)} \tilde{J}_{i' j', l}^{(n, \tilde{n})} S_{j', l}^{(\tilde{n})}. \quad (\text{S7})$$

If we further focus on the case  $n = \tilde{n}$ , these terms amount to a slightly modified version of a standard Heisenberg term, where the exchange matrix  $\tilde{\mathbf{J}}$  is a spatial modulation of the bare exchange in  $t_{2g}$  space. This modulation is due to the  $\mathbf{k}$ -dependent nature of the transformation  $S$  that defines the operators  $d^{(\dagger)}$ . By assuming an antiferromagnetic ordering of the moments in  $\alpha = 1/2$  space it can be shown that on top of this modulation all bare  $J$  values are reduced by a factor  $\sim \frac{1}{9}$ .

We are turning now to the exchange interactions in the  $t_{2g}$  space, which are given for the xz character of nearest neighbors in  $x$ -direction by  $J_{(xz, 1x)} = 4t_{1x}^2/U_{xz} = 0.18$  eV. Due to symmetry, they are the same for the yz character in  $y$ -direction ( $J_{(yz, 1y)}$ ), but further  $J_{i\alpha, j\alpha}$  elements with

$\alpha \in \{xz, yz\}$  are negligibly small. Here, we used hopping parameters  $t_\lambda$ , which were obtained from a tight-binding fit of the  $t_{2g}$  manifold, and on-site interactions  $U$ <sup>18</sup> calculated within the constrained random phase approximation (cRPA)<sup>19</sup>, both shown in Table 1. For the xy character we derive similarly  $J_{(xy,1)} = 4t_1^2/U_{xy} = 0.47$  eV. However, due to the extended nature of the xy component, the next-nearest neighbor contribution  $J_{(xy,2)} = 4t_2^2/U_{xy} = 0.16$  eV is rather large and only longer-ranged  $J_{i\ xy,j\ xy}$  can be ignored. It should be noted that if rescaled by the aforementioned factor  $\sim \frac{1}{9}$ , these parameters are in good agreement with values extracted from magnon dispersions using resonant inelastic x-ray spectroscopy<sup>14</sup>.

|                               | $\epsilon$ | $t_{1x}$                             | $t_{1y}$                            | $t_2$                                 |                                       | U   |
|-------------------------------|------------|--------------------------------------|-------------------------------------|---------------------------------------|---------------------------------------|-----|
| $d_{xz}$                      | -0.34      | 0.31                                 | 0.05                                | -0.01                                 |                                       | 2.1 |
| $d_{yz}$                      | -0.34      | 0.05                                 | 0.31                                | -0.01                                 |                                       | 2.1 |
| $\mathbf{R}_i - \mathbf{R}_j$ |            | $\pm \mathbf{e}_x$                   | $\pm \mathbf{e}_y$                  | $\pm \mathbf{e}_x \pm \mathbf{e}_y$   |                                       |     |
|                               | $\epsilon$ | $t_1$                                | $t_2$                               | $t_3$                                 | $t_4$                                 | U   |
| $d_{xy}$                      | -0.55      | 0.26                                 | 0.15                                | 0.06                                  | 0.05                                  | 0.6 |
| $\mathbf{R}_i - \mathbf{R}_j$ |            | $\pm \mathbf{e}_x, \pm \mathbf{e}_y$ | $\pm \mathbf{e}_x \pm \mathbf{e}_y$ | $\pm 2\mathbf{e}_x \pm 2\mathbf{e}_y$ | $\pm 3\mathbf{e}_x \pm 3\mathbf{e}_y$ |     |

Table 1: Real-space tight-binding parameterization of the  $t_{2g}$  hopping part and cRPA values<sup>18</sup> for the Coulomb repulsion  $U$  of the model. The corresponding vectors between sites  $i$  and  $j$  are listed as  $\mathbf{R}_i - \mathbf{R}_j$ . All values are in eV.

If we assume that we only have to retain these diagonal terms, the three components of  $\mathbf{J}$  are modeled differently. The  $xz$  and  $yz$  components are each described by a one-dimensional Heisen-

berg chain in  $x$ - and  $y$ -direction respectively, and hence order antiferromagnetically. However, the  $\alpha = xy$  component is described by the  $J_1$ - $J_2$ -Heisenberg model on the square lattice with  $J_2/J_1 \sim 1/3$ . This model is known to have a quantum disordered singlet ground state at zero temperature for  $0.4 \lesssim J_2/J_1 \lesssim 0.6$ , where quantum fluctuations prevent long-range ordering of the spins into an antiferromagnetic configuration<sup>15</sup>. With the ratio calculated above, in the present case the model is close to this state, which means that at finite temperatures small thermal fluctuations can be sufficient to destroy any putative antiferromagnetic zero temperature ground state and lead to a spin-disordered ground state instead.

Therefore, the  $d_{xy}$  spin components align along an external magnetic field, whereas the quasi-1D AF ordered spin components are less susceptible and give a weak response. As a result, the  $xy$ -component of the magnetization density follows the applied field and leads to a predominant  $xy$ -character as seen in the measurements.

In the reasoning above, the  $\mathbf{k}$ -dependent nature of the effective Wannier states is essential. If one assumes a given fixed composition of the  $j_{\text{eff}}$  orbital instead and formulates pseudospin-1/2 states, the weak ferromagnetism of the ground state is correctly captured<sup>16</sup>, but the application of a magnetic field does not change its composition and cannot explain the predominant  $xy$ -character of the magnetization density. Interestingly, *ab initio* calculations (DFT+SOC) revealed that the overall ( $\mathbf{k}$ -averaged)  $t_{2g}$  orbital composition of such a local  $j_{\text{eff}} = 1/2$  orbital does not deviate much from the isotropic composition of  $\frac{1}{\sqrt{3}} : \frac{1}{\sqrt{3}} : \frac{1}{\sqrt{3}}$  and, if anything, has a smaller contribution of the  $xy$ -orbital<sup>17</sup>. One should also note that the magnetic field strength of 5 T is too small to

explain why the WFM moment of a local  $j_{\text{eff}}$  state does not interlock with the octahedral rotation, but follows the direction of applied magnetic field instead. To capture the magnetization density distribution, it is therefore necessary to extend the standard description in terms of a static  $t_{2g}$  composition of the  $j_{\text{eff}} = 1/2$  state to a more realistic  $\mathbf{k}$ -dependent Wannier description  $\varphi_{\mathbf{k},\alpha}$  as proposed here.

## 7 References

1. Sung, N. *et al.* Crystal growth and intrinsic magnetic behaviour of  $\text{Sr}_2\text{IrO}_4$ . *Philosophical Magazine* **96**, 413–426 (2016).
2. Ye, F. *et al.* Magnetic and crystal structures of  $\text{Sr}_2\text{IrO}_4$ : A neutron diffraction study. *Physical Review B* **87**, 140406 (2013).
3. Dhital, C. *et al.* Neutron scattering study of correlated phase behavior in  $\text{Sr}_2\text{IrO}_4$ . *Physical Review B* **87**, 144405 (2013).
4. Fruchter, L., Colson, D. & Brouet, V. Magnetic critical properties and basal-plane anisotropy of  $\text{Sr}_2\text{IrO}_4$ . *Journal of Physics: Condensed Matter* **28**, 126003 (2016).
5. Nauman, M. *et al.* In-plane magnetic anisotropy in strontium iridate  $\text{Sr}_2\text{IrO}_4$ . *Physical Review B* **96**, 155102 (2017).
6. Hansen, N. K. & Coppens, P. Testing aspherical atom refinements on small-molecule data sets. *Acta Crystallographica Section A* **34**, 909–921 (1978).
7. Coppens, P. *X-ray charge densities and chemical bonding*, vol. 4 (International Union of Crystallography, Oxford University Press, (1997).
8. Paturle, A. & Coppens, P. Normalization factors for spherical harmonic density functions. *Acta Crystallographica Section A* **44**, 6–7 (1988).

9. Brown, P. & Matthewman, J. Ccsl, the cambridge crystallographic subroutine library. *Rutherford Appleton Laboratory, Rep. RAL-93-009* (1993).
10. Martins, C. Couplage Spin-Orbite et Interaction de Coulomb dans l'Iridate de Strontium  $\text{Sr}_2\text{IrO}_4$ . *PhD thesis, Ecole Polytechnique, Palaiseau* (2010).
11. Louat, A. *et al.* Orbital character and coherence energy scale defined by ARPES in Rh-doped  $\text{Sr}_2\text{IrO}_4$ . *in preparation* (2018).
12. Louat, A. Études spectroscopiques des nouveaux états électroniques induits par fort couplage spin-orbite dans les iridates. *PhD thesis, Université Paris-Saclay, Orsay* (2018).
13. Si, Q. & Abrahams, E. Strong Correlations and Magnetic Frustration in the High  $T_c$  Iron Pnictides. *Phys. Rev. Lett.* **101**, 076401 (2008).
14. Kim, J. *et al.* Magnetic Excitation Spectra of  $\text{Sr}_2\text{IrO}_4$  Probed by Resonant Inelastic X-Ray Scattering: Establishing Links to Cuprate Superconductors *Phys. Rev. Lett.* **112**, 177003 (2012).
15. Mambrini, M. *et al.* Plaquette valence-bond crystal in the frustrated Heisenberg quantum antiferromagnet on the square lattice. *Phys. Rev. B* **74**, 144422 (2006).
16. Wang, F. & Senthil, T. Twisted Hubbard Model for  $\text{Sr}_2\text{IrO}_4$ : Magnetism and Possible High Temperature Superconductivity. *Phys. Rev. Lett.* **106**, 136402 (2011).
17. Martins, C. *et al.* Coulomb correlations in 4d and 5d oxides from first principles – or how spin-orbit materials choose their effective orbital degeneracies. *J. Phys.: Condens. Matter* **29**, 263001 (2017).

18. Backes S., Jiang H. *et al.* unpublished.
19. Aryasetiawan F. *et al.* Frequency-dependent local interactions and low-energy effective models from electronic structure calculations *Phys. Rev. B* **70**, 195104 (2004).
